# Supplementary material for: SciExplore: Evaluating Autonomous Agents from Scientific Navigation to Information Integration
Source: arXiv:2607.20926 source file (2026-07-23)
Supplement: Supplementary file 1 [file appendix_vs_1.tex]

\begin{figure*}[!t]
            \centering
            \includegraphics[width=0.85\textwidth]{figs/imgs/1.pdf}
            \caption{\textbf{Visual comparison of baseline and AutoPage}. The webpage generated by the baseline (left) exhibits rendering failures, including an inability to display the formula and a distorted layout for images and tables. Conversely, the page generated by AutoPage (right) renders the formula correctly and preserves the intended layout of all visual elements.}
     \label{fig:app-visual_results1}
    \vspace{-10pt}
\end{figure*}
