# Supplementary material for: SciExplore: Evaluating Autonomous Agents from Scientific Navigation to Information Integration
Source: arXiv:2607.20926 source file (2026-07-23)
Supplement: Supplementary file 2 [file appendix_vs_2.tex]

\begin{figure*}[!t]

            \centering
            \includegraphics[width=0.82\textwidth]{figs/imgs/2.pdf}
            \caption{\textbf{Additional Visual comparison of baseline and AutoPage}. The baseline-generated page (left) suffers from improper image scaling, leading to a catastrophic visual presentation. In contrast, AutoPage (right) styles the tables to match the page's theme and displays the image at an optimal size.}
     \label{fig:app-visual_results2}
    \vspace{-10pt}
\end{figure*}
