# Supplementary material for: SciExplore: Evaluating Autonomous Agents from Scientific Navigation to Information Integration
Source: arXiv:2607.20926 source file (2026-07-23)
Supplement: Supplementary file 3 [file appendix_vs_3.tex]

\begin{figure*}[!t]

            \centering
            \includegraphics[width=0.82\textwidth]{figs/imgs/3.pdf}
            \caption{\textbf{Additional Visual comparison of baseline and AutoPage}. The webpage generated by the baseline method (left) fails to render the contents within their respective sections. Conversely, the page generated by AutoPage (right) successfully displays both the textual and visual elements in their correct layout.}
     \label{fig:app-visual_results3}
    \vspace{-10pt}
\end{figure*}
